# Supplementary material for: Breaking Rayleigh's law with spatially correlated disorder to control phonon transport
Source: arXiv:2308.10836 source file (2023-08-21)
Supplement: Supplementary file 1 [file supplementary_material.pdf]

# Supplementary Information: Breaking Rayleigh's law with spatially correlated disorder to control phonon transport

S. Thébaud, L. Lindsay, T. Berlijn

## 1 Details of the alloy model and generation of the correlated mass configurations

The model that we consider is a generic mass-disordered spring-mass system on a simple cubic lattice, with lattice constant  $a = 2.47 \text{ \AA}$ , average atomic masses  $m_0 = 50 \text{ amu}$  and nearest-neighbor interatomic force constants  $2.11 \text{ eV/\AA}$ . These parameters lead to a maximum angular frequency  $70 \text{ rad THz}$  and a sound velocity  $c = 5000 \text{ m/s}$  in the virtual crystal approximation (VCA), which is comparable to SiGe alloys [1]. We assume the vibrations along  $x$ ,  $y$  and  $z$  to be independent, so that only one direction is included in the calculations and a factor 3 is then added to the thermal conductivities.

The anharmonicity is taken into account through a frequency-dependent phonon-phonon Umklapp scattering rate

$$\frac{1}{\tau^U(\omega)} = A\omega^2 T e^{-\Theta/T} \quad (1)$$

with  $A = 3 \times 10^{-7} \text{ ps/K}$  and  $\Theta = 140 \text{ K}$ . These parameters are again similar to those evaluated in the literature from fitting thermal conductivity measurements of Si and Ge crystals [2, 1, 3], but also certain III-V semiconductors such as GaN [4]. In addition, they yield Umklapp scattering rates comparable to those calculated from first-principles in Si and GaAs [5, 6].

We create large supercells containing millions or tens of millions of atoms with correlated mass disorder configurations. Five atomic species with masses  $0.4m_0$ ,  $0.7m_0$ ,  $m_0$ ,  $1.3m_0$  and  $1.6m_0$  are distributed in the supercell with roughly equal concentrations. To produce the disorder configurations, we use a procedure close to that described in Ref [7]. We first generate an auxiliary continuous scalar field  $V(\mathbf{r})$  with the property that  $\frac{1}{N} \sum_{\mathbf{r}'} V(\mathbf{r}' + \mathbf{r}) V(\mathbf{r}') = C_{\text{target}}(\mathbf{r})$  where  $C_{\text{target}}(\mathbf{r})$  is the desired correlation function. Since the boundary conditions are periodic making the disorder-averaged field homogeneous, this ensures that  $\langle V(\mathbf{r}) V(\mathbf{0}) \rangle = C_{\text{target}}(\mathbf{r})$ . We then exploit the fact that the modulus square of the Fourier transform (FT) of the field is the FT of the correlation function. We thus compute the FT  $\tilde{C}_{\text{target}}(\mathbf{q})$  of  $C_{\text{target}}(\mathbf{r})$  by a fast Fourier transform (FFT) algorithm, then set the FT of the field as

$$\tilde{V}(\mathbf{q}) = \sqrt{\tilde{C}_{\text{target}}(\mathbf{q})} e^{i\varphi(\mathbf{q})} \quad (2)$$

where  $\varphi(\mathbf{q})$  are random phases that determine different configurations with the same target correlation function. Finally, we use a reverse FFT algorithm to compute  $V(\mathbf{r})$  and we discretize the field into five different values  $\delta m_{\mathbf{r}} = -0.6, -0.3, 0.0, 0.3$  and  $0.6$ . This generates a discrete mass distribution  $\delta m_{\mathbf{r}}$  whose correlation function  $C(\mathbf{r})$  is close to the desired correlation function  $C_{\text{target}}(\mathbf{r})$ . Note that this choice of 5 different species is strictly for convenience, any type of alloy can be considered.

## 2 Perturbative transport scattering rates

We start with the standard lowest-order perturbation formula for scattering of phonon mode  $\mathbf{k}$  by mass disorder [8, 9], corrected with a factor  $1 - \cos(\theta_{\mathbf{k}+\mathbf{q},\mathbf{k}})$  to account for the effectiveness of backward vs forward scattering,  $\theta_{\mathbf{k}+\mathbf{q},\mathbf{k}}$  being the angle between the velocities of modes  $\mathbf{k}$  and  $\mathbf{k} + \mathbf{q}$  (see e.g. chapter 16 of [10] or section 8.1.2 of [11]):

$$1/\tau_{\mathbf{k}}^{\text{tr}} = \frac{\pi}{\omega_{\mathbf{k}}} \sum_{\mathbf{q}} \langle |g_{\mathbf{q}}|^2 \rangle (1 - \cos(\theta_{\mathbf{k}+\mathbf{q},\mathbf{k}})) \delta(\omega_{\mathbf{k}+\mathbf{q}}^2 - \omega_{\mathbf{k}}^2). \quad (3)$$

$g_{\mathbf{q}}$  is the coupling matrix element between mode  $\mathbf{k}$  and  $\mathbf{k} + \mathbf{q}$ , whose disorder-averaged modulus square is given by the Fourier transform of the mass perturbation correlation function  $C(\mathbf{r}) = \langle \delta m_{\mathbf{r}} \delta m_{\mathbf{0}} \rangle$ :

$$\langle |g_{\mathbf{q}}|^2 \rangle = \omega^4 \frac{1}{N} \sum_{\mathbf{r}} C(\mathbf{r}) e^{-i\mathbf{q} \cdot \mathbf{r}}. \quad (4)$$

We will now show that correlation functions with power-law long-range decay have a Fourier transform that behaves as a power-law for small wavevectors, irrespective of the precise short-range behavior. Consider an isotropic correlation function that decreases like a power-law beyond a certain cutoff radius  $r_c$ :  $C(\mathbf{r}) = f(|\mathbf{r}|)$  with  $f(r) = \frac{B}{r^\alpha} e^{-r/\xi}$  for  $r > r_c$ , where a correlation length  $\xi$  has been introduced for regularization purposes and the limit  $\xi \rightarrow \infty$  will be taken at the end. Keeping only the contribution from the first Brillouin Zone since it is the dominant one at long wavelengths, the average coupling matrix element is given by

$$\langle |g_{\mathbf{q}}|^2 \rangle = \frac{\omega^4}{(2\pi a)^3} \int_{\mathbb{R}^3} d^3\mathbf{r} f(|\mathbf{r}|) e^{-i\mathbf{q} \cdot \mathbf{r}} \quad (5)$$

$$= \frac{\omega^4}{2\pi^2 a^3 q} \int_0^\infty dr r f(r) \sin(qr) \quad (6)$$

$$= \frac{\omega^4}{2\pi^2 a^3 q} \int_0^{r_c} dr r f(r) \sin(qr) + \frac{\omega^4}{2\pi^2 a^3 q} \int_{r_c}^\infty dr \frac{B}{r^{\alpha-1}} e^{-r/\xi} \sin(qr). \quad (7)$$

Since  $f(0) = \langle \delta m^2 \rangle$  is finite, the first term, short-ranged, is bounded as  $q \rightarrow 0$ . As we will see, the other term diverges if  $\alpha < 3$ . Therefore, we will ignore the first term and focus on the long-ranged term. Introducing the rescaling  $u = qr$  yields

$$\langle |g_{\mathbf{q}}|^2 \rangle = \frac{B\omega^4}{2\pi^2 a^3 q^{3-\alpha}} \int_{qr_c}^\infty du \frac{\sin(u)}{u^{\alpha-1}} e^{-u/q\xi}. \quad (8)$$

For  $\alpha \geq 1$ , the integral converges straightforwardly when  $\xi \rightarrow \infty$  and  $\langle |g_{\mathbf{q}}|^2 \rangle$  behaves as  $1/q^{3-\alpha}$  for small  $q$ . For  $0 < \alpha < 1$ , it is helpful to express the sine as a sum of two complex exponentials and then perform an integration by parts:

$$\langle |g_{\mathbf{q}}|^2 \rangle = \frac{B\omega^4}{2\pi^2 a^3 q^{3-\alpha} 2i} \left( \int_{qr_c}^\infty du u^{1-\alpha} e^{(i-1/q\xi)u} - \int_{qr_c}^\infty du u^{1-\alpha} e^{(-i-1/q\xi)u} \right) \quad (9)$$

$$= \frac{B\omega^4}{2\pi^2 a^3 q^{3-\alpha} 2i} \left( -\frac{(qr_c)^{1-\alpha} e^{(i-1/q\xi)qr_c}}{i - \frac{1}{q\xi}} - \frac{1-\alpha}{i - \frac{1}{q\xi}} \int_{qr_c}^\infty du \frac{e^{(i-1/q\xi)u}}{u^\alpha} \right. \\ \left. + \frac{(qr_c)^{1-\alpha} e^{(-i-1/q\xi)qr_c}}{-i - \frac{1}{q\xi}} + \frac{1-\alpha}{-i - \frac{1}{q\xi}} \int_{qr_c}^\infty du \frac{e^{(-i-1/q\xi)u}}{u^\alpha} \right) \quad (10)$$

$$= \frac{B\omega^4}{2\pi^2 a^3 q^{3-\alpha}} \left( (qr_c)^{1-\alpha} e^{-r_c/\xi} \frac{\cos(qr_c) + \frac{1}{q\xi} \sin(qr_c)}{1 + \frac{1}{q^2 \xi^2}} \right. \\ \left. + \frac{1-\alpha}{1 + \frac{1}{q^2 \xi^2}} \int_{qr_c}^\infty du e^{-u/q\xi} \frac{\cos(u) + \frac{1}{q\xi} \sin(u)}{u^\alpha} \right). \quad (11)$$

In the  $\xi \rightarrow \infty$  limit, the term in parentheses converges to  $(qr_c)^{1-\alpha} \cos(qr_c) + (1-\alpha) \int_{qr_c}^{\infty} du \frac{\cos(u)}{u^\alpha}$ , which remains bounded for small  $q$ . Thus, in this case also  $\langle |g_{\mathbf{q}}|^2 \rangle$  behaves as  $1/q^{3-\alpha}$  for small  $q$ .

We then calculate the long-wavelength transport scattering rate from equation (3), assuming a Debye dispersion  $\omega_{\mathbf{k}} = c||\mathbf{k}||$  which is valid at low  $q$ . Due to the delta function imposing  $||\mathbf{k}|| = ||\mathbf{k}+\mathbf{q}||$ , the correction factor  $1-\cos(\theta_{\mathbf{k}+\mathbf{q},\mathbf{k}})$  becomes  $q^2/2k^2$  and the transport scattering rate is

$$1/\tau_{\mathbf{k}}^{\text{tr}} \propto \frac{1}{\omega_{\mathbf{k}}} \int d^3\mathbf{q} \frac{\omega_{\mathbf{k}}^4}{q^{3-\alpha}} \frac{q^2}{2k^2} \delta(c^2(\mathbf{k}+\mathbf{q})^2 - c^2\mathbf{k}^2) \quad (12)$$

$$\propto k \int d^3\mathbf{q} q^{\alpha-1} \delta(c^2q^2 + 2c^2\mathbf{k} \cdot \mathbf{q}) \quad (13)$$

$$\propto k \int_0^{q_D} dq q^{1+\alpha} \int_0^\pi d\theta \sin(\theta) \delta(q^2 + 2kq \cos(\theta)) \quad (14)$$

$$\propto k \int_0^{q_D} dq q^{1+\alpha} \int_{-1}^1 du \delta(q^2 + 2kqu) \quad (15)$$

$$\propto \int_0^{2k} dq q^\alpha \quad (16)$$

$$\propto k^{1+\alpha}. \quad (17)$$

We thus find that the transport scattering decreases as  $\omega^{1+\alpha}$  instead of the usual  $\omega^4$ . It is interesting to note that, for the usual perturbative expression without the  $1-\cos(\theta_{\mathbf{k}+\mathbf{q},\mathbf{k}})$  factor, the integral (16) becomes  $\int_0^{2k} q^{\alpha-2}$ , which diverges for  $\alpha \leq 1$ . It is then necessary to perform a self-consistent Born approximation as in e.g. Ref. [12]. Thus, accounting for backscattering through the correction factor is crucial in the presence of correlations, and the single-particle phonon linewidths give only limited information about the thermal transport properties.

### 3 Phonon spectral function and transport formalism

Our methods based on the phonon Green's function formalism have been detailed elsewhere [13, 14, 15], but for convenience we will give a brief presentation here. The phonon Green's function of a harmonic disordered supercell containing  $N$  sites can be defined as

$$\mathbf{G}(\omega) = \frac{1}{(\omega + i\eta)^2 - \mathbf{D}} \quad (18)$$

where  $\mathbf{D} = \frac{1}{\sqrt{\mathbf{M}}} \mathbf{\Phi} \frac{1}{\sqrt{\mathbf{M}}}$  is the dynamical matrix.  $\mathbf{M}$  is the diagonal matrix of the atomic masses,  $\mathbf{\Phi}$  is the matrix of the interatomic force constants and  $\eta$  is a real positive infinitesimal. In the present case, the disorder on the force constants are neglected, thus only  $\mathbf{M}$  and  $\mathbf{D}$  are disordered.  $\mathbf{G}(\omega)$  is the Fourier transform of the correlation function of the mass-renormalized atomic displacement operators [14].

The spectral function for the plane-wave phonon mode with wavevector  $\mathbf{k}$  can be defined as

$$A(\mathbf{k}, \omega) = -\frac{2\omega}{\pi} \text{Im} \langle E_{\mathbf{k}} | \sqrt{\frac{\mathbf{M}_0}{\mathbf{M}}} \mathbf{G}(\omega) \sqrt{\frac{\mathbf{M}_0}{\mathbf{M}}} | E_{\mathbf{k}} \rangle \quad (19)$$

where  $|E_{\mathbf{k}}\rangle = \frac{1}{\sqrt{N}} \sum_{\mathbf{r}} e^{i\mathbf{k} \cdot \mathbf{r}} |\mathbf{r}\rangle$  and  $\mathbf{M}_0$  is the VCA (disorder-averaged) mass matrix. We remind the reader that the bra-ket notation is used here strictly for convenience, as the vectors denote atomic degrees of freedom and not actual quantum states of the phonon Fock space. That being said, the Green's function formalism used here is fully quantum mechanical. When  $A(\mathbf{k}, \omega)$

exhibits a well-defined peak as a function of frequency (well-defined phonon quasiparticle), the central frequency corresponds to the disorder-renormalized phonon frequency and the full-width at half maximum (FWHM) corresponds to the disorder-limited inverse lifetime of the mode.

The Green-Kubo formalism provides a quantum linear-response expression for the thermal conductivity that fully incorporates disorder effects, including the important ladder vertex corrections associated with the backscattering  $1 - \cos(\theta)$  factor [11], and does not rely on well-defined phonon quasiparticles:

$$\kappa = \int_0^\infty d\omega W_{\text{ph}}(\omega) \frac{\pi k_B^2 T}{3\hbar\Omega} \text{Tr} \left[ \text{Im}\mathbf{G}(\omega + \frac{i}{2\tau^{\text{U}}(\omega)}) \mathbf{S} \text{Im}\mathbf{G}(\omega + \frac{i}{2\tau^{\text{U}}(\omega)}) \mathbf{S} \right] \quad (20)$$

where  $T$  is the temperature,  $\Omega$  is the supercell volume,  $\mathbf{S}_{\mathbf{r},\mathbf{r}'} = \frac{1}{i}(\mathbf{r} - \mathbf{r}')D_{\mathbf{r},\mathbf{r}'}$  is the Hardy heat current operator [16] and  $W_{\text{ph}} = \frac{3}{\pi^2} \left( \frac{\hbar\omega}{k_B T} \right)^2 \left( -\frac{\partial f_B}{\partial \omega} \right)$  acts as a normalized half-window of width  $\approx 2k_B T$  centered on  $\omega = 0$ , with  $f_B$  the Bose-Einstein distribution. The Umklapp phonon-phonon interactions are taken into account as the frequency-dependent inverse lifetime  $\frac{1}{\tau^{\text{U}}(\omega)}$  playing the role of an inelastic damping in the phonon Green's function. This approach is broadly equivalent to that recently used for amorphous solids by Isaeva [17], except that we evaluate expression (20) using the CPGF method (see section 4) instead of diagonalizing the dynamical matrix, which allows us to reach very large system sizes up to tens of millions of sites.

We also compute the thermal conductivity along direction  $x$  using the standard kinetic expression

$$\kappa = \frac{1}{\Omega} \sum_{\mathbf{k}} c_v(\omega_{\mathbf{k}}) v_{x,\mathbf{k}}^2 \tau_{\mathbf{k}}^{\text{tr,tot}} \quad (21)$$

where  $c_v(\omega) = \hbar\omega \frac{\partial f_B}{\partial T}(\omega)$  is the heat capacity of phonon modes with frequency  $\omega$ ,  $v_{x,\mathbf{k}}$  is the velocity of mode  $\mathbf{k}$  along  $x$ .  $\tau_{\mathbf{k}}^{\text{tr,tot}}$  is the total transport lifetime of mode  $\mathbf{k}$ , given by Matthiessen's rule:

$$\frac{1}{\tau_{\mathbf{k}}^{\text{tr,tot}}} = \frac{1}{\tau_{\mathbf{k}}^{\text{tr}}} + \frac{1}{\tau^{\text{U}}(\omega_{\mathbf{k}})} \quad (22)$$

with  $\tau_{\mathbf{k}}^{\text{tr}}$  the phonon-disorder transport scattering rate defined in section 2 and  $1/\tau^{\text{U}}$  the phonon-phonon Umklapp scattering rate defined in section 1.

At low frequencies, the Green-Kubo conductivity calculations become very costly (see next section) but give the same contribution to  $\kappa$  as the standard kinetic expression using the transport lifetime, because the phonon quasiparticle picture is essentially valid at these low frequencies. Thus, we use the full Green-Kubo method only above 10 rad THz, and we complement it with the simpler kinetic expression below 10 rad THz. Therefore, the dots in Fig. 4 of the main text are obtained strictly speaking from a mix of Green-Kubo CPGF and kinetic theory calculations. The dashed curve, however, are entirely obtained from kinetic theory at all frequencies.

## 4 The Chebyshev polynomial Green's function method

The Chebyshev polynomials Green's function (CPGF) method has been reviewed in Refs. [18, 19] for electrons, and has been adapted in Refs. [15, 14, 13] for phonons. The central idea is to efficiently evaluate equations (19) and (20) by expanding the phonon Green's function on the Chebyshev polynomial basis:

$$\mathbf{G}(\bar{\omega}) = \sum_{n=0}^{\infty} g_n ((\bar{\omega} + i\bar{\eta})^2) T_n(\bar{\mathbf{D}}) \quad (23)$$

where the bar indicates that the spectrum has been rescaled to  $[-1, 1]$ , the  $g_n(z)$  are known complex functions:

$$g_n(z) = -i(2 - \delta_{n,0}) \frac{(z - i\sqrt{1-z^2})^n}{\sqrt{1-z^2}} \quad (24)$$

and the  $T_n(\bar{\mathbf{D}})$  are Chebyshev polynomials evaluated for the dynamical matrix, that follow the recursion relation  $T_{n+1}(\bar{\mathbf{D}}) = 2\bar{\mathbf{D}}T_n(\bar{\mathbf{D}}) - T_{n-1}(\bar{\mathbf{D}})$  with  $T_1(\bar{\mathbf{D}}) = \bar{\mathbf{D}}$  and  $T_0(\bar{\mathbf{D}}) = 1$ . Equality (23) comes from the identity

$$e^{-izt} = \sum_{n=0}^{\infty} \frac{2i^{-n}}{1 + \delta_{n,0}} J_n(t) T_n(z) \quad (25)$$

for  $|z| < 1$  with  $J_n(t)$  the Bessel function of order  $n$  (see equations (5) through (9) in the supplementary material of Ref. [18]).

Since the spectral function for the Bloch mode  $\mathbf{k}$  is given by eq. (19), the quantities to be calculated are the so-called moments  $\mu_{n,\mathbf{k}}$ :

$$\mu_{n,\mathbf{k}} = \langle E_{\mathbf{k}} | \sqrt{\frac{\mathbf{M}_0}{\mathbf{M}}} T_n(\bar{\mathbf{D}}) \sqrt{\frac{\mathbf{M}_0}{\mathbf{M}}} | E_{\mathbf{k}} \rangle, \quad (26)$$

which are computed using the recursion relation between the  $T_n(\bar{\mathbf{D}})$ . Once this is done, the spectral function can be obtained at any  $\omega$  at virtually no computational cost. The number of moments necessary for the sum (23) to converge is roughly equal to  $1/2\bar{\omega}\bar{\eta}$ . Because  $\bar{\eta}$  is an artificial broadening and should be smaller than the disorder-induced spectral linewidth, probing modes closer and closer to  $\Gamma$  requires more and more polynomials to be included. To extract the phonon lifetimes of low-frequency modes, we calculate up to  $10^6$  moments on supercells  $305 \times 305 \times 305$ . For such system sizes, only one disorder configuration is necessary except when very long-range  $1/\sqrt{r}$  are present, in which case we use 4 different configurations to ensure a proper disorder average.

The trace in equation 20 can be called the phonon transport distribution function (TDF)  $\Sigma_{\text{ph}}(\omega)$ . To calculate it, we use the one-shot stochastic procedure described in Ref. [13, 18]:

$$\Sigma_{\text{ph}}(\omega) = \frac{\pi k_B^2 T}{3\hbar\Omega} \frac{1}{N_r} \sum_{\lambda} \langle \varphi_-^{\lambda} | \varphi_+^{\lambda} \rangle \quad (27)$$

with  $|\varphi_+^{\lambda}\rangle = \text{Im}\mathbf{G}(\omega + \frac{i}{2\tau\bar{v}(\omega)})\mathbf{S}|\lambda\rangle$  and  $|\varphi_-^{\lambda}\rangle = \mathbf{S}\text{Im}\mathbf{G}(\omega + \frac{i}{2\tau\bar{v}(\omega)})|\lambda\rangle$ .  $N_r$  random vectors  $|\lambda\rangle = \sum_{\mathbf{r}} e^{i\varphi_{\mathbf{r}}} |\mathbf{r}\rangle$  are defined, with  $\varphi_{\mathbf{r}}$  a random phase uniformly distributed in the interval  $[0, 2\pi]$ . The vectors  $|\varphi_+^{\lambda}\rangle$  and  $|\varphi_-^{\lambda}\rangle$  are calculated iteratively for every frequency above 10 rad THz and every temperature. At low frequencies, the Umklapp scattering rates become smaller and smaller, leading to an ever increasing number of terms to be calculated for the Chebyshev series (23) to converge. This is why we rely instead on the simpler kinetic formula below 10 rad THz. Above 10 rad THz, we calculate up to 120000 terms in the series (23) on supercells of size  $1200 \times 200 \times 200$ . The larger size along the transport direction  $x$  allows us to reach the thermodynamic limit by avoiding ballistic effects. We use two disorder configurations for  $1/\sqrt{r}$  and  $1/r$  correlations, and one configuration for  $1/r^2$  correlations and the uncorrelated case.

## 5 Acoustic phonon spectral functions

We show here in Fig. S1 the phonon spectral function of selected acoustic modes from Fig 3 of the main text in the relevant frequency range (0 to 35 rad THz). They have been calculated from the CPGF method, and the spectral peak broadenings are representative of the disorder-induced lifetime of each mode. Extracting the FWHM of low-frequency modes is computationally difficult for two main reasons:

- The number of terms (moments) that must be included in the Chebyshev expansion (23) of the Green's function is proportional to  $\frac{1}{\omega\eta}$ , with  $\omega$  the mode angular frequency and  $\eta$  an artificial broadening that must be much smaller than the mode FWHM. Because the linewidth is proportional to  $\omega^2$  for  $1/r$  correlations and to  $\omega^4$  for the uncorrelated case, the number of moments that must be calculated grows as  $1/\omega^3$  for  $1/r$  correlations and as  $1/\omega^5$  for the uncorrelated case.
- Finite-size effects (i.e. the separation between discrete levels of the disordered system) must be small compared to the mode FWHM, implying that the supercell size must grow as  $1/\omega^2$  and  $1/\omega^4$  for  $1/r$  correlations and no correlations respectively. Computational time is linear with the system size in the CPGF method, but so is memory space. Also, it should be kept in mind that the cubic symmetry in the clean system considered leads to a 48-fold degeneracy for most  $\mathbf{k}$ -points, which increases the level separation substantially. Strictly speaking, these degeneracies are lifted by disorder but this is a small effect at low frequencies.

Of note, the CPGF algorithm relies on an iterative procedure whose parallelization overheads quickly limits the gain obtained from using multiple CPUs. In addition, we have been quite strict when it comes to convergence and have shown only those data points for which we could ascertain that finite size effects are small enough and the number of moments high enough to make the results reliable. From these considerations, we encounter a computational wall at low frequencies. To give an example, the lowest-frequency point shown in Fig. 3 for the uncorrelated case (around 10 rad THz), has been calculated on a  $305 \times 305 \times 305$  supercell with  $10^6$  moments. The calculation for this mode alone took two weeks and around 150GB of RAM. To go lower in frequency would have required both more moments and a larger system, leading to steep costs in both time and memory. For systems featuring spatial correlations, we are more limited by finite-size effects than by the number of moments. Fortunately, the power-law trends are already quite clear in Fig. 3 of the main text, making it unnecessary to go to lower frequencies. We also want to emphasize that the FWHM of the lowest frequency modes shown in Fig. 3 are completely unreachable through exact diagonalization, given the system sizes of several tens of millions of atoms required to calculate them reliably.

## 6 Numerical evaluation of the thermal conductivity

We show in Fig S2 the same data as in Fig. 4 of the main text in logarithmic scale to emphasize the differences in the values of  $\kappa$  predicted for the various correlation power-laws. In this figure, it is also apparent that perturbative estimates of  $\kappa$  are slightly underestimated compared to CPGF estimates. This is partly due to the fact that the perturbative expression used here does not include the phonon diffusive channel [20]. As mentioned in section 2, if the vertex correction factor  $1 - \cos(\theta_{\mathbf{k}+\mathbf{q},\mathbf{k}})$  is omitted for correlations decaying slower than  $1/r$ , the second-order perturbative scattering rates diverge. Numerically, this leads to a non-convergence of the scattering rates as the number of  $\mathbf{k}$ -points increases and the broadening  $\eta$  of the delta peaks in eq (3) decreases. For a given broadening parameter, the scattering rate calculated in this way is also higher than the transport scattering rate (which includes the vertex correction factor) by order of magnitudes. Thus, omitting the vertex correction factor in the perturbative evaluation of  $\kappa$  would lead to a gross overestimation: in the case of  $1/\sqrt{r}$  correlations, for instance, the value obtained for the room-temperature thermal conductivity would be  $0.075 \text{ W m}^{-1} \text{ K}^{-1}$  instead of  $2.63 \text{ W m}^{-1} \text{ K}^{-1}$ . It is clear that vertex corrections are absolutely crucial to capturing the physics of thermal transport in the presence of spatial correlations.

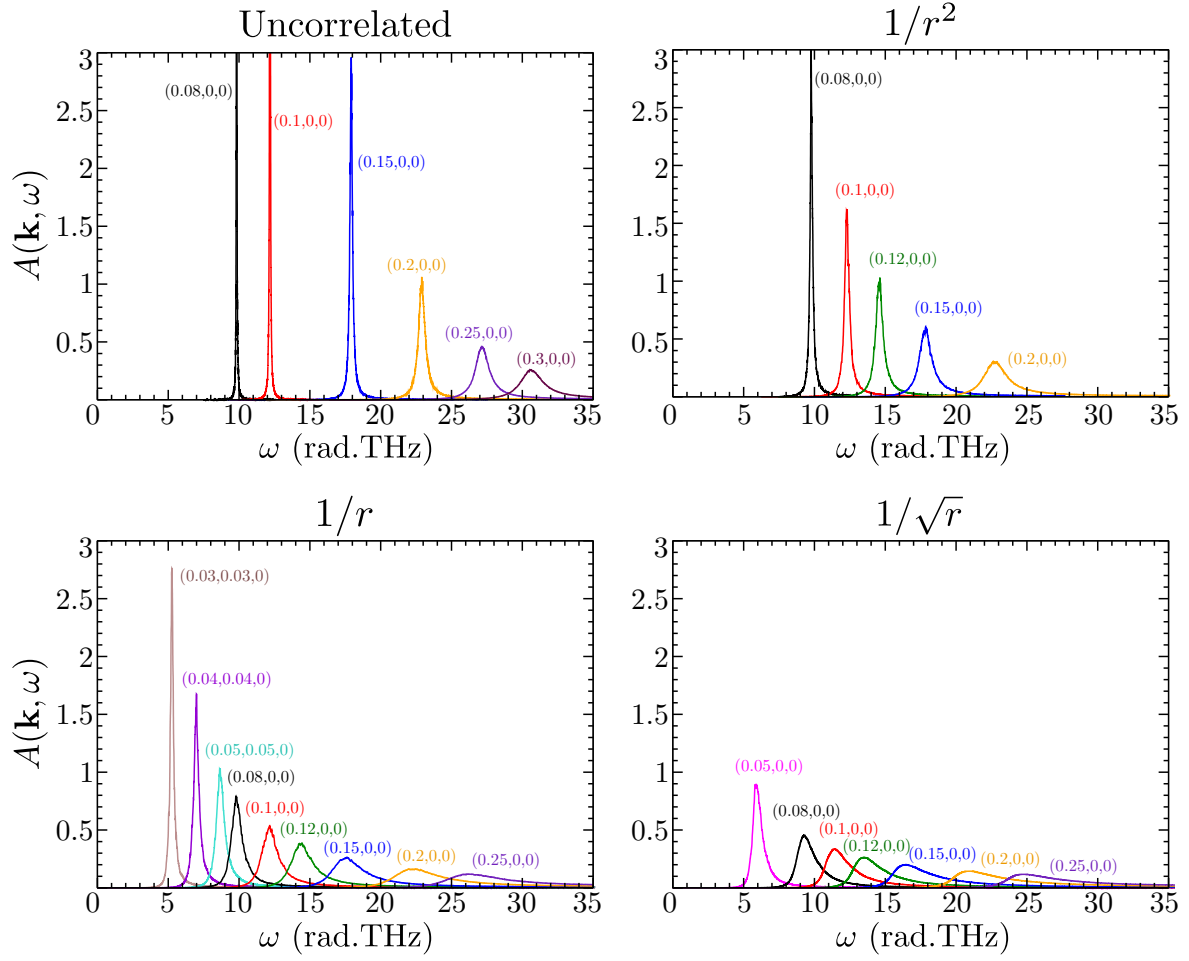

Figure S1: Phonon-spectral function of acoustic modes for several power-law decaying correlations  $C(\mathbf{r}) \propto 1/r^\alpha$  with  $\alpha = \infty$  (uncorrelated) and  $\alpha = 2, 1$ , and  $0.5$ . The curve labels  $(k_x, k_y, k_z)$  are the mode wavevectors in units of  $2\pi/a$ .

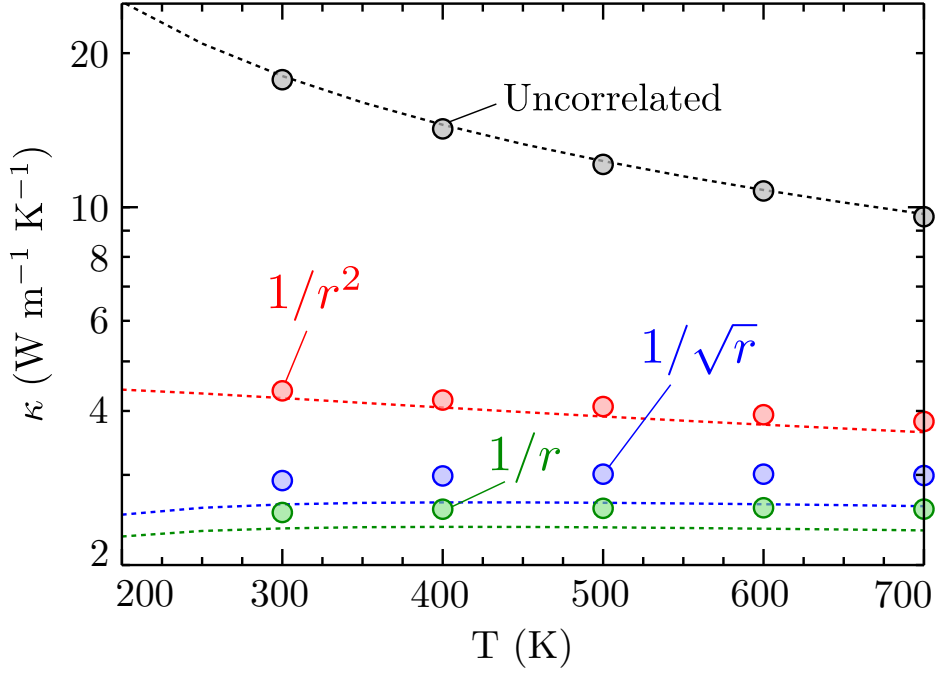

Figure S2: The thermal conductivities for several power-law decaying correlations evaluated through Green-Kubo CPGF calculations above 10 rad THz, with second-order perturbation theory below 10 rad THz (dots) and through perturbation theory only (dashed lines).

## 7 Optimal correlations to minimize $\kappa$

To find the optimal correlation that minimizes the thermal conductivity, we make the fundamental assumption that the simple kinetic expressions (21) and (22) (including the  $1 - \cos(\theta)$  vertex correction factor in the disorder scattering rates) are valid. This assumption is supported by our numerical results (Fig. 4 of the main text).  $\kappa$  then depends on the mass correlations through the phonon-disorder transport scattering rate (see equations (3) and (4)):

$$1/\tau_{\mathbf{k}}^{\text{tr}} = \pi \omega_{\mathbf{k}}^3 \int \frac{d^3 \mathbf{q}}{(2\pi)^3} \Omega \tilde{C}(\mathbf{q}) (1 - \cos(\theta_{\mathbf{k}+\mathbf{q}, \mathbf{k}})) \delta(\omega_{\mathbf{k}+\mathbf{q}}^2 - \omega_{\mathbf{k}}^2), \quad (28)$$

where  $\tilde{C}(\mathbf{q}) = \frac{1}{N} \sum_{\mathbf{r}} C(\mathbf{r}) e^{-i\mathbf{q} \cdot \mathbf{r}}$  is the FT of the correlation function. We then minimize the thermal conductivity as a functional of  $\tilde{C}(\mathbf{q})$  while keeping the disorder strength  $C(\mathbf{0}) = \int \frac{d^3 \mathbf{q}}{(2\pi)^3} \Omega \tilde{C}(\mathbf{q})$  constant. This constraint eliminates the obvious solution of introducing more and more disorder, instead answering the question: given a certain amount of defects or disorder, how best to organize it spatially to impede the flow of heat?

Introducing a Lagrange multiplier  $\lambda$ , we are to solve

$$\frac{\delta}{\delta \tilde{C}(\mathbf{q})} \left[ \int \frac{d^3 \mathbf{k}}{(2\pi)^3} c_v(\omega_{\mathbf{k}}) v_{x,\mathbf{k}}^2 \tau_{\mathbf{k}}^{\text{tr,tot}} - \lambda \int \frac{d^3 \mathbf{k}}{(2\pi)^3} \Omega \tilde{C}(\mathbf{k}) \right] = 0. \quad (29)$$

Since

$$\frac{\delta \tau_{\mathbf{k}}^{\text{tr,tot}}}{\delta \tilde{C}(\mathbf{q})} = -(\tau_{\mathbf{k}}^{\text{tr,tot}})^2 \pi \omega_{\mathbf{k}}^3 \frac{\Omega}{(2\pi)^3} (1 - \cos(\theta_{\mathbf{k}+\mathbf{q}, \mathbf{k}})) \delta(\omega_{\mathbf{k}+\mathbf{q}}^2 - \omega_{\mathbf{k}}^2), \quad (30)$$

we obtain

$$\pi \int \frac{d^3 \mathbf{k}}{(2\pi)^3} c_v(\omega_{\mathbf{k}}) v_{x,\mathbf{k}}^2 \omega_{\mathbf{k}}^3 (\tau_{\mathbf{k}}^{\text{tr,tot}})^2 (1 - \cos(\theta_{\mathbf{k}+\mathbf{q}, \mathbf{k}})) \delta(\omega_{\mathbf{k}+\mathbf{q}}^2 - \omega_{\mathbf{k}}^2) = -\lambda. \quad (31)$$

To make more analytical progress, we now assume a Debye dispersion  $\omega_{\mathbf{k}} = c||\mathbf{k}||$ . Due to isotropy, the left-hand side  $f_x$  of equation (31) does not depend on the transport direction considered:  $f_x = f_y = f_z = (f_x + f_y + f_z)/3$ . Thus:

$$\frac{\pi}{3} \int \frac{d^3\mathbf{k}}{(2\pi)^3} c_v(\omega_{\mathbf{k}}) c^5 ||\mathbf{k}||^3 (\tau_{\mathbf{k}}^{\text{tr,tot}})^2 \frac{||\mathbf{q}||^2}{2||\mathbf{k}||^2} \delta(c^2(\mathbf{k} + \mathbf{q})^2 - c^2\mathbf{k}^2) = -\lambda. \quad (32)$$

Introducing spherical coordinate with  $\theta$  the angle between  $\mathbf{k}$  and  $\mathbf{q}$ :

$$\frac{c^3 q^2}{24\pi} \int_0^{k_D} dk c_v(\omega_k) k^3 (\tau_k^{\text{tr,tot}})^2 \int_0^\pi d\theta \sin(\theta) \delta(2kq \cos(\theta) + q^2) = -\lambda, \quad (33)$$

where  $k_D$  is the Debye wavevector. The angular integral of the delta function simplifies to  $\Theta(2k - q)/(2kq)$  with  $\Theta$  the Heaviside function, so we have:

$$\frac{c^3 q}{48\pi} \int_{q/2}^{k_D} dk c_v(\omega_k) k^2 (\tau_k^{\text{tr,tot}})^2 = -\lambda. \quad (34)$$

Moving the prefactor to the right-hand side and taking the derivative on both sides with respect to  $q$  then yields:

$$-\frac{1}{2} c_v(\omega_{q/2}) (q/2)^2 (\tau_{q/2}^{\text{tr,tot}})^2 = \frac{48\pi\lambda}{c^3 q^2}. \quad (35)$$

Finally, substituting  $q/2 \rightarrow q$  we obtain

$$\frac{1}{\tau_q^{\text{tr,tot}}} = \sqrt{\frac{c^3 c_v(\omega_q)}{24\pi|\lambda|}} q^2, \quad (36)$$

as asserted in the main text.

## 8 Finite correlation length

In order to evaluate the impact of a finite correlation length that would make the correlations short-ranged, we calculate the phonon-disorder transport scattering rates and the thermal conductivities for a correlation function of the form  $C(\mathbf{r}) \propto \frac{1}{r} e^{-r/\xi}$ . Such an  $r$  dependence arises naturally in the context of an Ising system, for instance. We make use of the Fermi golden rule to calculate the transport scattering rates (equation (3) and (4)), and we evaluate the thermal conductivity through kinetic theory (equation (21) and (22)). Fig. 4 of the main text shows this methodology to be in excellent agreement with a full Green-Kubo treatment of the thermal conductivity.

We show in Fig S1 the phonon-disorder transport scattering rates for  $\xi = 0$  (reference case without correlation),  $\xi = 2.47 \text{ \AA}$ ,  $4.94 \text{ \AA}$ ,  $12.35 \text{ \AA}$ ,  $24.70 \text{ \AA}$ ,  $49.40 \text{ \AA}$  (1, 2, 5, 10, 20 lattice constants respectively) and  $\xi = \infty$  corresponding to optimal  $1/r$  correlations. For finite correlation lengths, the low-frequency scattering rates always follow an  $\omega^4$  Rayleigh law as the phonon wavelength is much greater than the typical cluster length. At intermediate frequencies, there is a crossover towards an  $\omega^2$  as the wavelength becomes comparable to the cluster size. However, even for very small correlation lengths down to a few Angströms, the scattering rates are substantially increased at low frequencies compared to the uncorrelated case.

The associated thermal conductivities are shown in Fig S4. Even for  $\xi$  equal to one lattice constant,  $\kappa$  is halved compared to the uncorrelated case. The optimal  $1/r$  thermal conductivity is recovered as soon as  $\xi$  equals 5 to 10 lattice constants. Thus, the inevitable presence of a finite correlation range in actual samples does not seem to be a serious obstacle to manipulating  $\kappa$  through disorder correlations.

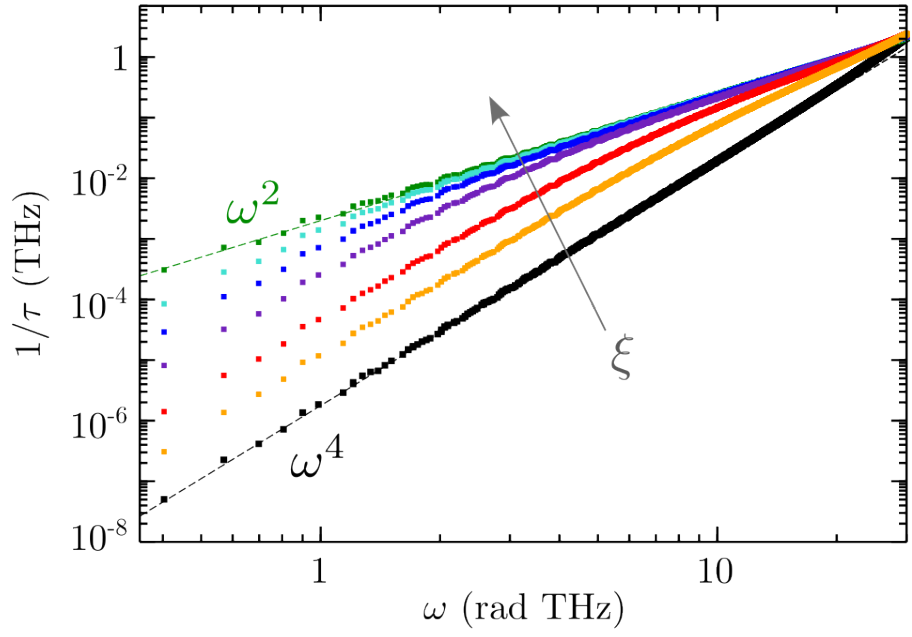

Figure S3: Phonon-disorder transport scattering rates from lowest-order perturbation theory for several values of the correlation length  $\xi = 0$  (black, no correlation),  $a$  (orange),  $2a$  (red),  $5a$  (purple),  $10a$  (blue),  $20a$  (cyan) and  $\xi = \infty$  (green).

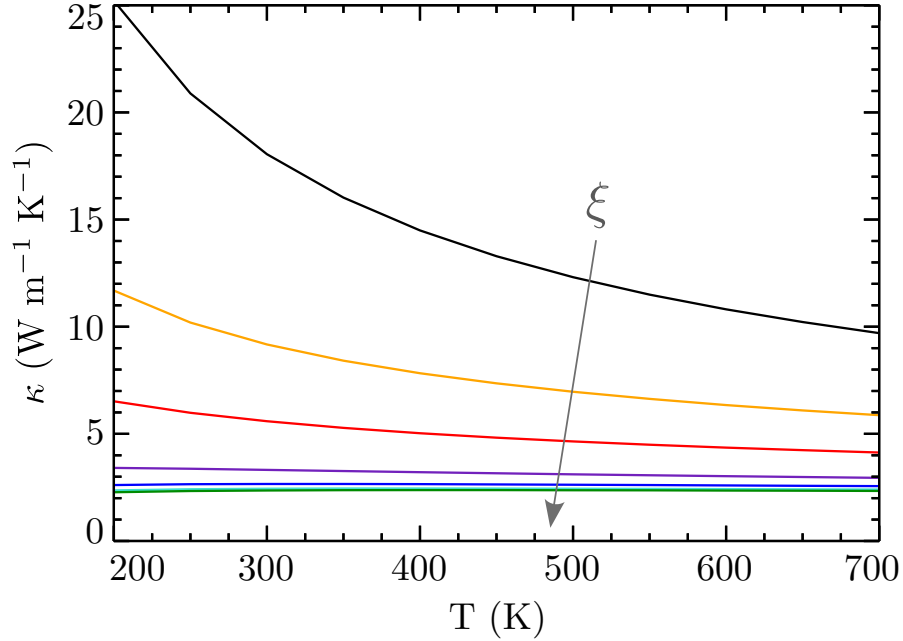

Figure S4: The thermal conductivities evaluated through second-order perturbation theory for several values of the correlation length  $\xi = 0$  (black, no correlation),  $a$  (orange),  $2a$  (red),  $5a$  (purple),  $10a$  (blue),  $20a$  (cyan) and  $\xi = \infty$  (green).

# References

- [1] Changwook Jeong, Supriyo Datta, and Mark Lundstrom. Full dispersion versus Debye model evaluation of lattice thermal conductivity with a Landauer approach. *Journal of Applied Physics*, 109(7):073718, April 2011.
- [2] N. Mingo. Calculation of Si nanowire thermal conductivity using complete phonon dispersion relations. *Physical Review B*, 68(11):113308, September 2003.
- [3] M. Asen-Palmer, K. Bartkowski, E. Gmelin, M. Cardona, A. P. Zhernov, A. V. Inyushkin, A. Taldenkov, V. I. Ozhogin, K. M. Itoh, and E. E. Haller. Thermal conductivity of germanium crystals with different isotopic compositions. *Physical Review B*, 56(15):9431–9447, October 1997.
- [4] Csaba Guthy, Chang-Yong Nam, and John E. Fischer. Unusually low thermal conductivity of gallium nitride nanowires. *Journal of Applied Physics*, 103(6):064319, March 2008.
- [5] Tengfei Luo, Jivtesh Garg, Junichiro Shiomi, Keivan Esfarjani, and Gang Chen. Gallium arsenide thermal conductivity and optical phonon relaxation times from first-principles calculations. *EPL (Europhysics Letters)*, 101(1):16001, January 2013.
- [6] Jivtesh Garg, Nicola Bonini, Boris Kozinsky, and Nicola Marzari. Role of Disorder and Anharmonicity in the Thermal Conductivity of Silicon-Germanium Alloys: A First-Principles Study. *Physical Review Letters*, 106(4):045901–045901, January 2011.
- [7] F. M. Izrailev and N. M. Makarov. Anomalous transport in low-dimensional systems with correlated disorder. *Journal of Physics A: Mathematical and General*, 38(49):10613–10637, November 2005.
- [8] Shin-ichiro Tamura. Isotope scattering of dispersive phonons in Ge. *Physical Review B*, 27(2):858–866, January 1983.
- [9] Shin-ichiro Tamura. Isotope scattering of large-wave-vector phonons in GaAs and InSb: Deformation-dipole and overlap-shell models. *Physical Review B*, 30(2):849–854, July 1984.
- [10] N W Ashcroft and N D Mermin. *Solid State Physics*. Saunders College, 1976.
- [11] G D Mahan. *Many Particle Physics, Third Edition*. Plenum, New York, 2000.
- [12] Sajeed John and Michael J. Stephen. Wave propagation and localization in a long-range correlated random potential. *Physical Review B*, 28(11):6358–6368, December 1983.
- [13] S. Thébaud, T. Berlijn, and L. Lindsay. Perturbation theory and thermal transport in mass-disordered alloys: Insights from Green’s function methods. *Physical Review B*, 105(13):134202, April 2022.
- [14] S. Thébaud, C. A. Polanco, L. Lindsay, and T. Berlijn. Success and breakdown of the T-matrix approximation for phonon-disorder scattering. *Physical Review B*, 102(9):094206, September 2020.
- [15] G. Bouzerar, S. Thébaud, S. Pecoraro, and Ch. Adessi. Drastic effects of vacancies on phonon lifetime and thermal conductivity in graphene. *Journal of Physics: Condensed Matter*, 32(29):295702, April 2020.
- [16] Robert J Hardy. Energy-Flux Operator for a Lattice. *Physical Review*, 132(1):168–177, October 1963.
- [17] Leyla Isaeva, Giuseppe Barbalinardo, Davide Donadio, and Stefano Baroni. Modeling heat transport in crystals and glasses from a unified lattice-dynamical approach. *Nature Communications*, 10:3853, August 2019.
- [18] Aires Ferreira and Eduardo R Mucciolo. Critical Delocalization of Chiral Zero Energy Modes in Graphene. *Physical Review Letters*, 115(10):106601–106601, August 2015.
- [19] Alexander Weiße, Gerhard Wellein, Andreas Alvermann, and Holger Fehske. The kernel polynomial method. *Reviews of Modern Physics*, 78(1):275–306, March 2006.
- [20] Michele Simoncelli, Nicola Marzari, and Francesco Mauri. Unified theory of thermal transport in crystals and glasses. *Nature Physics*, 15(8):809–813, August 2019.
